# Supplementary material for: Risk-sensitive safety analysis using Conditional Value-at-Risk
Source: arXiv:2101.12086 source file (2022-06-25)
Supplement: Supplementary file 2 [file old_appendix.tex]

To prove Theorem \ref{thm33}, we require the following lemma.
\begin{lemma}[Measurability of Multi-Mapping]\label{lemma5}
Let $Y : \mathbb{R} \rightarrow \mathbb{R}$ be a bounded and Borel measurable function. Under Assumptions \ref{assumption0}-\ref{assumption2}, the function\vspace{-2mm}
\begin{equation} \label{eq_multi}
\vspace{-1mm}\begin{aligned}
x_{t-1} \hspace{-1mm} \mapsto \hspace{-1mm}
 \sup_{\xi_t \in \mathcal{R}_{\alpha,t}^\pi(x_{t-1})}  \textstyle\int_{\mathbb{R}} Q(\mathrm{d}x_t |x_{t-1},\pi_{t-1}(x_{t-1})) \xi_t(x_t) Y(x_t)
\end{aligned}\vspace{-1mm}
\vspace{-1mm}\end{equation}
is bounded and Borel measurable.
\end{lemma}

The key reason for Assumptions \ref{assumption0}-\ref{assumption2} is to prove Lemma \ref{lemma5}, which is done in the Supplementary Material due to space constraints.
\textcolor{white}{begin proof}\\
\indent \marginnote{\textcolor{black}{\textbf{R4 C3e}}}{ Next,} we prove Theorem \ref{thm33}.\\
\begin{proof}[Thm. \ref{thm33} \emph{(\textcolor{blue}{Dynamic Programming} to Upper Bound $\rho_{\alpha,x}^\pi$)}]
The function $J_T = c_T$ is bounded and Borel measurable since $c_T$ has these properties. Suppose that for some $t = 1,\dots,T$, $J_t$ is bounded and Borel measurable. Then, $J_{t-1}$ \eqref{Jtminus1} is bounded and Borel measurable by Lemma \ref{lemma5} and since $c_{t-1}$ is bounded and Borel measurable. Hence, by induction, the functions $J_t$ for all $t =0,\dots,T$ are bounded and Borel measurable. Now, the expectation of $Y$ with respect to $\bar{P}_x^\pi \in \mathcal{D}_{\alpha,x}^\pi$ is\vspace{-2mm}
\begin{equation*}\begin{aligned}
     \textstyle \int_{\mathbb{R}^{T+1}}  Y \mathrm{d}\bar{P}_x^\pi
    &  \textstyle =  \int_{\mathbb{R}^{T+1}}  Y \xi^{x_0}_1 \cdots \xi^{x_{T-1}}_T \mathrm{d}P_x^\pi\\
    &  \textstyle =  \int_{\mathbb{R}}  \delta_x(\mathrm{d} x_0) \int_{\mathbb{R}}  Q(\mathrm{d} x_1|x_0,\pi_0(x_0)) \xi^{x_0}_1(x_1) \cdots \\
    &  \textstyle \textcolor{white}{==}  \int_{\mathbb{R}} Q(\mathrm{d} x_T|{ x_{T-1},\pi_{T-1}(x_{T-1})}) \xi^{x_{T-1}}_{T}(x_T)\\
    &  \textstyle \textcolor{white}{==}   \big( c_T(x_T) +\textstyle \sum_{t=0}^{T-1} c_t(x_t,\pi_t(x_t)) \big),
\end{aligned}\end{equation*}
where $P_x^\pi$ refers to \eqref{54b}.
We can separate the above expression into parts, where each part does not depend on the entire state history (due to the ``separable'' structure of the random cost $Y$ and the probability measure $\bar{P}_x^\pi$, and since $\pi$ is a Markov policy). We show this expression for $T=3$ for clarity below:\vspace{-1mm}
\begin{equation}\label{73}\begin{aligned}
    & \textstyle \int_{\mathbb{R}^{T+1}} Y \mathrm{d}\bar{P}_x^\pi \\
    & = \textstyle c_0(x,\pi_0(x)) + \int_{\mathbb{R}}  Q(\mathrm{d} x_1|x,\pi_0(x)) \xi^{x}_{1}(x_{1}) \Big( c_1(x_1,\pi_1(x_1)) + \\
    & \textstyle \textcolor{white}{=} \int_{\mathbb{R}}  Q(\mathrm{d} x_2|x_1,\pi_1(x_1)) \xi^{x_1}_{2}(x_{2}) \Big( c_2(x_2,\pi_2(x_2)) + \\ & \textstyle \textcolor{white}{=} \int_{\mathbb{R}}  Q(\mathrm{d} x_3|x_2,\pi_2(x_2)) \xi^{x_2}_3(x_3) c_3(x_3) \Big) \Big),
\end{aligned}\vspace{-1mm}\end{equation}
where we used the definition of the Dirac measure $\delta_x$ (the distribution of $X_0$ is concentrated at $x \in \mathbb{R}$). We will show the inequality \eqref{upperbound} for $T = 3$ to facilitate readability of the argument, which generalizes to $T \in \mathbb{N}$ by using induction. Since $T = 3$, we have $J_3 = c_3$, and the function $J_2 : \mathbb{R} \rightarrow \mathbb{R}$\vspace{-1mm}
\begin{equation}\label{74}\begin{aligned}
    J_2(x_2) & := c_2(x_2,\pi_2(x_2)) \\
    & + \sup_{\xi_3 \in \mathcal{R}_{\alpha,3}^\pi(x_{2})} \textstyle  \int_{\mathbb{R}}  Q(\mathrm{d} x_3|x_2,\pi_2(x_2)) \xi_3(x_3) J_3(x_3).
\end{aligned} \vspace{-1mm} \end{equation}
is bounded and Borel measurable. Eqs. \eqref{73} and \eqref{74} imply \vspace{-1mm} 
\begin{equation}\label{75}\begin{aligned}
& \textstyle \int_{\mathbb{R}^{T+1}} Y \mathrm{d}\bar{P}_x^\pi\\
& \textstyle \leq c_0(x,\pi_0(x)) + \int_{\mathbb{R}}  Q(\mathrm{d} x_1|x,\pi_0(x)) \xi^{x}_{1}(x_{1}) \Big( c_1(x_1,\pi_1(x_1)) \\
    & \textstyle \textcolor{white}{=} + \int_{\mathbb{R}}  Q(\mathrm{d} x_2|x_1,\pi_1(x_1)) \xi^{x_1}_{2}(x_{2}) J_2(x_2) \Big).
\end{aligned}\vspace{-1mm} \end{equation}
% Now, we use Lusin's Theorem to provide a continuous approximation of $J_2$, which is non-negative. Let $\epsilon > 0$ and $x_1 \in \mathbb{R}$. \textcolor{red}{Let $\xi_2 \in \mathcal{R}_{x,\alpha,t}^\pi(x_{1})$. Then, $J_2 \in  L^\infty(\mathbb{R},\mathcal{B}(\mathbb{R}), Q(\cdot|x_1,\pi_1(x_1))\xi_2)$ because [please fill in].} By Lusin's Theorem \textcolor{red}{(what is the precise statement, we should write this down)}, there exists a continuous function $J_2^\epsilon : \mathbb{R} \rightarrow \mathbb{R}$ such that
% \begin{equation}\begin{aligned}
%     & \int_{\mathbb{R}} Q(\mathrm{d} x_2|x_1,\pi_1(x_1)) \xi_2(x_2) J_2(x_2) \\
%     & \leq \frac{\epsilon ||J_2||_{L^\infty}}{\alpha^{T+1}} + \int_{\mathbb{R}} Q(\mathrm{d} x_2|x_1,\pi_1(x_1)) \xi_2(x_2) J_2^\epsilon(x_2)\\
%     & \leq \frac{\epsilon ||J_2||_{L^\infty}}{\alpha^{T+1}} + \hspace{-2mm} \sup_{\xi_2 \in \mathcal{R}_{x,\alpha,t}^\pi(x_{1})} \hspace{-0.5mm} \int_{\mathbb{R}} \hspace{-1mm} Q(\mathrm{d} x_2|x_1,\pi_1(x_1)) \xi_2(x_2) J_2^\epsilon(x_2).
% \end{aligned}\end{equation}
% The upper bound is Borel measurable by Lemma \ref{lemma5} since $J_2^\epsilon$ is continuous. $||\cdot||_{L^\infty}$ is the norm on \textcolor{red}{ $L^\infty(\mathbb{R},\mathcal{B}(\mathbb{R}), Q(\cdot|x_1,\pi_1(x_1)))$? It doesn't make sense that the norm depends on $x_1$?}
Now, $J_1 : \mathbb{R} \rightarrow \mathbb{R}$ is bounded and Borel measurable
\begin{equation}\label{77}\begin{aligned}
    % J_1(x_1) & := c_1(x_1,\pi_1(x_1)) + \frac{\epsilon ||J_2||_{L^\infty}}{\alpha^{T+1}}\\ 
    % & + \sup_{\xi_2 \in \mathcal{R}_{x,\alpha,t}^\pi(x_{1})}  \int_{\mathbb{R}}  Q(\mathrm{d} x_2|x_1,\pi_1(x_1)) \xi_2(x_2) J_2^\epsilon(x_2).
    J_1(x_1) & := c_1(x_1,\pi_1(x_1)) \\ 
    & + \sup_{\xi_2 \in \mathcal{R}_{\alpha,2}^\pi(x_{1})}  \textstyle \int_{\mathbb{R}}  Q(\mathrm{d} x_2|x_1,\pi_1(x_1)) \xi_2(x_2) J_2(x_2).
\end{aligned}\vspace{-1mm}\end{equation}
Equations \eqref{75} and \eqref{77} imply
\begin{equation}\label{633}\begin{aligned}
\int_{\mathbb{R}^{T+1}} \hspace{-4mm} Y \mathrm{d}\bar{P}_x^\pi \hspace{-.5mm} \leq\hspace{-.5mm}  c_0(x,\pi_0(x))  + \hspace{-1.5mm}\int_{\mathbb{R}} \hspace{-1.5mm} Q(\mathrm{d} x_1|x,\pi_0(x)) \xi^{x}_{1}(x_{1}) J_1(x_1).
\end{aligned}\end{equation} 
Finally, $J_0 : \mathbb{R} \rightarrow \mathbb{R}$ is bounded and Borel measurable\vspace{-2mm}
\begin{equation}\label{622}\begin{aligned}
    J_0(x) & := c_0(x,\pi_0(x)) \\ 
    & + \sup_{\xi_1 \in \mathcal{R}_{\alpha,1}^\pi(x)}  \textstyle \int_{\mathbb{R}}  Q(\mathrm{d} x_1|x,\pi_0(x)) \xi_{1}(x_{1}) J_1(x_1).
\end{aligned}\vspace{-1mm}\end{equation}
Equations \eqref{633} and \eqref{622} imply $\int_{\mathbb{R}^{T+1}} Y \mathrm{d}\bar{P}_x^\pi \leq J_0(x)$. Since the above analysis holds for any $\bar P^{\pi}_x \in \mathcal{D}^{\pi}_{\alpha,x}$, we have\vspace{-2mm}
\begin{equation}\label{64}
\rho_{\alpha,x}^\pi(Y) := \underset{\bar P^{\pi}_x \in \mathcal{D}^{\pi}_{\alpha,x}}{\sup} \textstyle\int_{\mathbb{R}^{T+1}} Y \mathrm{d}\bar{P}_x^\pi \leq J_0(x).\vspace{-2mm}
\end{equation}
Eq. \eqref{64} holds for any $x \in \mathbb{R}$, $\alpha \in (0,1]$, and $\pi \in \Pi_M$ since these were chosen arbitrarily (recall the text of Sec. \ref{sectheory}).
\end{proof}

%\begin{remark}[$\xi_t^*$ lacks regularity]
%Following this remark, we prove Theorem \ref{thm33} by induction. For the sake of discussion, suppose that for some $t \in \{0,1,\dots,T-1\}$, $J_{t+1}^\alpha$ is lsc, bounded, and non-negative. Define $\phi_t^\alpha : S \times A \rightarrow \mathbb{R}$ by
%\begin{equation*}
%\phi_t^\alpha(x,u) :=  \sup_{\xi(\cdot|x,u) \in \mathcal{R}_{\alpha}(x,u)} \textstyle \int_{S} J_{t+1}^\alpha(y) \textcolor{blue}{\xi(y|x,u)} Q(\mathrm{d} y|x,u).
%\end{equation*}
%By Lemma \ref{attainmentlemma}, for any $(x,u) \in S \times A$, there is a $\xi_t^*(\cdot|x,u) \in \mathcal{R}_\alpha(x,u)$ such that
%\begin{equation}\begin{aligned}
%    $\phi_t^\alpha(x,u) = \textstyle \int_{S}   J_{t+1}^\alpha(y) \xi_t^*(y|x,u) Q(\mathrm{d} y|x,u)$.
%\end{aligned}\end{equation}
%For any $y \in S$, the map $(x,u) \mapsto \xi_t^*(y|x,u)$ need \emph{not} be Borel measurable because the set-valued mapping $(x,u) \mapsto \mathcal{R}_{\alpha}(x,u)$ need not be sufficiently regular. It follows that $\phi_t^\alpha$ need not be Borel measurable. In the literature, this issue is circumvented by adopting a more general framework, in which a supremum is taken over a set $B(x,u)$ such that the set-valued mapping $(x,u) \mapsto B(x,u)$ is assumed to be lower semi-continuous \cite[Assumption 3.1 (g), p. 1632]{trejo2002}. A similar approach is used in \cite[Thm. 2, Condition (ii), p. 246]{ruszczynski2010risk}. Unfortunately, we cannot make such claims about $(x,u) \mapsto \mathcal{R}_{\alpha}(x,u)$. However, we can use $\nu^\alpha$, a Borel measurable and bounded function that does not depend on $(x,u)$. For any $\xi(\cdot|x,u) \in \mathcal{R}_\alpha(x,u)$, it holds that $0 \leq \xi(\cdot|x,u) J_{t+1}^\alpha \leq \nu^\alpha J_{t+1}^\alpha$ a.e. w.r.t. $Q(\cdot|x,u)$. We use strong continuity of $Q$ and Borel measurability of $\nu^\alpha$, in particular, to ensure that $\varphi_t^\alpha$ \eqref{varphit} is Borel measurable in the following proof.
%\end{remark}

\begin{proof}[Thm. \ref{thm33}]
Proceed by induction. $J_T^\alpha = c_T$ is lsc, bounded, and non-negative. Now, assume that for some $t \in \{0,1,\dots,T-1\}$, $J_{t+1}^\alpha$ is lsc, bounded, and non-negative. Since $J_{t+1}^\alpha \nu^\alpha$ is a product of Borel measurable and bounded functions, and $Q$ is strongly continuous, the function $\varphi_t^\alpha : S \times A \rightarrow \mathbb{R}$, $\varphi_t^\alpha(x,u) := \textstyle \int_{S} J_{t+1}^\alpha(y) \nu^\alpha(y) Q(\mathrm{d} y|x,u)$, is continuous and bounded.
%\textcolor{red}{By Assumption \ref{assumption3}, $\xi_t^\alpha(y|x,u)Q(\mathrm{d}y|x,u)$ is a continuous stochastic kernel on $S$ given $S \times A$. From this and $J_{t+1}^\alpha$ being lsc and bounded, it follows that $\phi_t^\alpha$ is lsc and bounded on $S \times A$ by \cite[Prop. 7.31(a), p. 148]{bertshreve2004}.} 
Since $\varphi_t^\alpha$ and $c_t$ are lsc, bounded, and non-negative, $v_t^\alpha = c_t + \varphi_t^\alpha$ is as well. Since $v_t^\alpha$ is lsc and $A$ is compact, $J_t^\alpha$ is lsc, and there is a Borel measurable function $\kappa_t^\alpha : S \rightarrow A$ such that
\begin{equation}\label{importantstep}
    J_t^\alpha(x) = v_t^\alpha(x,\kappa_t^\alpha(x)) \;\;\; \forall x \in S
\end{equation}
by \cite[Prop. 7.33, p. 153]{bertshreve2004}. Boundedness and non-negativity of $J_t^\alpha$ follows from boundedness and non-negativity of $v_t^\alpha$. Define $\pi_\alpha^* := (\kappa_0^\alpha, \dots,\kappa_{T-1}^\alpha)$.

Next, we show \eqref{upperbound}. Let $\Pi'$ be the set of randomized Markov policies. Since $\inf_{\pi \in \Pi} \rho_{\alpha,x}^\pi(Y) \leq \inf_{\pi \in \Pi'} \rho_{\alpha,x}^\pi(Y)$, it suffices to upper bound the latter quantity. For $t = 0,1,\dots,T$, define the random cost-to-go by $Y_t := c_T(X_T) + \sum_{i=t}^{T-1} c_i(X_i,U_i)$ if $t < T$; $Y_t := c_T(X_T)$ if $t = T$. Note that 
%\begin{equation}
%    Y_t := \begin{cases} c_T(X_T) + \sum_{i=t}^{T-1} c_i(X_i,U_i) & \text{ if }t<T \\ c_T(X_T) & \text{ if }t=T \end{cases},
%\end{equation}
$Y = Y_0$. For any $\pi := (\pi_0,\dots,\pi_{T-1}) \in \Pi'$ and $\zeta := (\xi_0,\dots,\xi_{T-1}) \in \mathcal{D}_\alpha$, denote the $(\pi,\zeta)$-conditional expectation of $Y_t$ given $X_t$ by $W_t^{\pi,\zeta}(x) := E^{\pi,\zeta}(Y_t|X_t = x)$, where $x \in S$. Note that $W_0^{\pi,\zeta}(x) = \int_{\Omega} Y \xi_0 \cdots \xi_{T-1} \mathrm{d}P_x^\pi$ for any $x \in S$, and thus,
\begin{equation}\label{my55}
    \rho_{\alpha,x}^\pi(Y) = \sup_{\zeta \in \mathcal{D}_\alpha} W_0^{\pi,\zeta}(x)\;\;\; \forall x \in S.
\end{equation}
Since $\pi_\alpha^* \in \Pi'$, it holds that
\begin{equation}\label{my56}
   \inf_{\pi \in \Pi'} \rho_{\alpha,x}^\pi(Y) \leq \rho_{\alpha,x}^{\pi_\alpha^*}(Y) \overset{\eqref{my55}}{=} \sup_{\zeta \in \mathcal{D}_\alpha} W_0^{\pi_\alpha^*,\zeta}(x)\;\;\; \forall x \in S.
\end{equation}
Now, if $W_0^{\pi_\alpha^*,\zeta}(x) \leq J_0^\alpha(x)$ for all $x \in S$ and $\zeta \in \mathcal{D}_\alpha$, then
%\begin{equation}
    $\underset{\zeta \in \mathcal{D}_\alpha}{\sup} W_0^{\pi_\alpha^*,\zeta}(x) \leq J_0^\alpha(x)$ for all $x \in S$.
%\end{equation}
This would complete the proof via \eqref{my56} and $\inf_{\pi \in \Pi} \rho_{\alpha,x}^\pi(Y) \leq \inf_{\pi \in \Pi'} \rho_{\alpha,x}^\pi(Y)$. Hence, it suffices to show that
%\begin{equation}
   $W_t^{\pi_\alpha^*, \zeta}(x) \leq J_t^\alpha(x)$ for all $x \in S$, $t \in \{0,1,\dots,T\}$, and $\zeta \in \mathcal{D}_\alpha$.
%\end{equation}
The base case holds because $W_T^{\pi_\alpha^*, \zeta} = c_T = J_T^\alpha$ for all $\zeta \in \mathcal{D}_\alpha$. Now, assume (the induction hypothesis) that for some $t \in \{0,1,\dots,T-1\}$, it holds that $W_{t+1}^{\pi_\alpha^*, \zeta} \leq J_{t+1}^\alpha$ for all $\zeta \in \mathcal{D}_\alpha$.
%For $t=T$, we have $W_T^{\pi,\zeta} = c_T$. %For $t = 0,1,\dots,T-1$, it holds that
%\begin{equation}\begin{aligned}
%    & W_t^{\pi,\zeta}(x_t) \\
%    & \textstyle \hspace{-1mm} = \hspace{-1mm}\int_A \int_S \int_A \cdots \int_S \Big( c_T(x_T) + \sum_{i=t}^{T-1} c_i(x_i,u_i) \Big) \\
 %   & \hphantom{=} \xi_T(x_T|x_{T-1},u_{T-1}) Q(\mathrm{d}x_T|x_{T-1},u_{T-1}) \cdots \\
 %    & \hphantom{=} \pi_{t+1}(\mathrm{d}u_{t+1}|x_{t+1}) \xi_t(x_{t+1}|x_t,u_t) Q(\mathrm{d}x_{t+1}|x_t,u_t) \pi_t(\mathrm{d}u_t|x_t).
%\end{aligned}\end{equation}
%for all $x_t \in S$. 
For any $\pi \in \Pi'$ and $\zeta \in \mathcal{D}_\alpha$, by deriving the form of $W_t^{\pi,\zeta}$, the following recursion (``law of iterated expectations'') holds: for $t = 0,1,\dots,T-1$ and $x \in S$,
\begin{subequations}\label{iterated}
\begin{equation}
     W_t^{\pi,\zeta}(x) 
      = \textstyle \int_A \Big( c_t(x,u) +  \psi_{t}^{\pi,\zeta}(x,u) \Big) \pi_t(\mathrm{d}u|x),
\end{equation}
where $\psi_{t}^{\pi,\zeta}$ is defined in terms of $W_{t+1}^{\pi,\zeta}$, $\xi_t$, and $Q$,
\begin{equation}
    \psi_{t}^{\pi,\zeta}(x,u) := \textstyle \int_S W_{t+1}^{\pi,\zeta}(y)\;\xi_t(y|x,u)\; Q(\mathrm{d}y|x,u)
\end{equation}
\end{subequations}
for all $(x,u) \in S \times A$. Let $x \in S$ and $\zeta \in \mathcal{D}_\alpha$. By expressing \eqref{iterated} for $\pi = \pi_\alpha^*$, a deterministic policy, it follows that
\begin{equation}\label{60}
    W_t^{\pi_\alpha^*,\zeta}(x) 
    = c_t(x,\kappa_t^\alpha(x)) +  \psi_{t}^{\pi_\alpha^*,\zeta}(x,\kappa_t^\alpha(x)).
\end{equation}
Note that the final term in \eqref{60} is given by
%\begin{equation*}
 $ \psi_{t}^{\pi_\alpha^*,\zeta}(x,\kappa_t^\alpha(x))  = \textstyle \int_S W_{t+1}^{\pi_\alpha^*,\zeta}(y)\xi_t(y|x,\kappa_t^\alpha(x)) Q(\mathrm{d}y|x,\kappa_t^\alpha(x))$.  
%\end{equation*}
By using the induction hypothesis, Borel measurability of $W_{t+1}^{\pi_\alpha^*,\zeta}$, $J_{t+1}^\alpha$, and $\xi_t(\cdot|x,\kappa_t^\alpha(x))$, a.e.-non-negativity of $\xi_t(\cdot|x,\kappa_t^\alpha(x))$ and $W_{t+1}^{\pi_\alpha^*,\zeta}$, we have
\begin{equation*}
  \psi_{t}^{\pi_\alpha^*,\zeta}(x,\kappa_t^\alpha(x)) 
   \leq \textstyle \int_S J_{t+1}^\alpha(y)\;\xi_t(y|x,\kappa_t^\alpha(x))\; Q(\mathrm{d}y|x,\kappa_t^\alpha(x)).
\end{equation*}
Since $0 \leq J_{t+1}^\alpha\xi_t(\cdot|x,\kappa_t^\alpha(x)) \leq J_{t+1}^\alpha\nu^\alpha$ a.e., it follows that
\begin{equation}\label{66}\begin{aligned}
    \psi_{t}^{\pi_\alpha^*,\zeta}(x,\kappa_t^\alpha(x)) & \leq \textstyle \int_S J_{t+1}^\alpha(y)\;\nu^\alpha(y)\; Q(\mathrm{d}y|x,\kappa_t^\alpha(x)) \\ & = \varphi_t^\alpha(x,\kappa_t^\alpha(x)).
\end{aligned}\end{equation}
By \eqref{60} and \eqref{66},
%\begin{equation}
    $W_t^{\pi_\alpha^*,\zeta}(x) \leq c_t(x,\kappa_t^\alpha(x)) + \varphi_t^\alpha(x,\kappa_t^\alpha(x))$.
%\end{equation}
Since $v_t^\alpha = c_t + \varphi_t^\alpha$ and by using \eqref{importantstep}, we conclude that
%\begin{equation}
    $W_t^{\pi_\alpha^*,\zeta}(x) \leq v_t^\alpha(x,\kappa_t^\alpha(x)) \overset{\eqref{importantstep}}{=} J_t^\alpha(x)$.
%\end{equation}
Since $x \in S$ and $\zeta \in \mathcal{D}_\alpha$ are arbitrary, the induction is complete.
%Since \eqref{62} holds for any $x \in S$ and $\zeta \in \mathcal{D}_\alpha$, the proof is complete.
\end{proof}

%Let $(x,u) \in S \times A$, and fix the probability space $(S, \mathcal{B}(S), Q(\cdot|x,u))$. That is, $L^p$ refers to $L^p(S, \mathcal{B}(S), Q(\cdot|x,u))$. The terms weak and weakly refer to the weak topology $\sigma(L^1,L^\infty)$.
%It suffices to show that $\mathcal{R}_{\alpha}(x,u)$ is compact in the weak topology and the functional $\nu : \mathcal{R}_{\alpha}(x,u) \rightarrow \mathbb{R}$ defined by \begin{equation}
%    \nu(\xi(\cdot|x,u)) := \textstyle \int_{S} J(y) \xi(y|x,u) Q(\mathrm{d} y|x,u)
%\end{equation}
%is continuous in the weak topology. We view $\mathcal{R}_{\alpha}(x,u)$ as the set of random variables $\xi(\cdot|x,u)$ in $L^1$ such that $\xi(y|x,u) \in [0,\alpha^{\frac{-1}{T}}]$ \textcolor{red}{for all $y \in S$} and $\int_S \xi(y|x,u) Q(\mathrm{d}y|x,u) = 1$. We view $J$ as a random variable in $L^\infty$. It follows that $\nu$ is weakly continuous.\footnote{Let $\{\xi_n(\cdot|x,u)\} \subseteq L^1$ converge weakly to $\xi(\cdot|x,u) \in L^1$. That is, $\lim_{n \rightarrow \infty} \int_S \xi_n(y|x,u) v(y) Q(\mathrm{d} y|x,u) = \int_S \xi(y|x,u) v(y) Q(\mathrm{d} y|x,u)$ for any $v \in L^\infty$. Since $J \in L^\infty$, it holds that $\lim_{n \rightarrow \infty} \nu(\xi_n(\cdot|x,u)) = \nu(\xi(\cdot|x,u))$.} To show that $\mathcal{R}_{\alpha}(x,u)$ is weakly compact, first note that $\mathcal{R}_{\alpha}(x,u)$ is uniformly bounded, which implies that $\mathcal{R}_{\alpha}(x,u)$ is uniformly integrable. The latter property implies that $\mathcal{R}_{\alpha}(x,u)$ is relatively weakly compact by the Dunford-Pettis Compactness Criterion \cite[p. 27-II]{typewriter}. That is, there is a set $\mathcal{R}'(x,u)$ such that 
%\begin{itemize}
 %   \item $\mathcal{R}_\alpha(x,u) \subseteq \mathcal{R}'(x,u) \subseteq L^1$, and
  %  \item $\mathcal{R}'(x,u)$ is compact in the weak topology $\sigma(L^1,L^\infty)$.
%\end{itemize}
%Recall that $S$ is a Borel space, which implies that it is separable. Since $\mathcal{R}'(x,u) \subseteq L^1$ is weakly compact and \textcolor{red}{$S$ is separable}, it holds that $\mathcal{R}'(x,u)$ is metrizable and weakly sequentially compact by a special case of the Eberlein-$\check{\text{S}}$mulian Theorem \cite[p. 26-II]{typewriter}.\footnote{$\mathcal{R}'(x,u)$ being \emph{weakly sequentially compact} means that every sequence in $\mathcal{R}'(x,u)$ contains a subsequence that converges weakly to an element of $\mathcal{R}'(x,u)$.} \textcolor{red}{It follows that $\mathcal{R}_\alpha(x,u) \subseteq \mathcal{R}'(x,u)$ is weakly closed}.\footnote{$\mathcal{R}_\alpha(x,u) \subseteq \mathcal{R}'(x,u)$ being \emph{weakly closed} means that for any sequence in $\mathcal{R}_\alpha(x,u)$ that converges weakly to an element $\xi(\cdot|x,u) \in \mathcal{R}'(x,u)$, it holds that $\xi(\cdot|x,u) \in \mathcal{R}_\alpha(x,u)$.} Finally, since a closed subset of a compact topological space is compact \cite[Prop. 4.22, p. 128]{folland2013real}, it follows that $\mathcal{R}_\alpha(x,u)$ is weakly compact.

%$\mathcal{R}_\alpha(x,u)$ is weakly closed. Since $\mathcal{R}_\alpha(x,u)$ is a convex subset of $L^2$, it suffices to show that $\mathcal{R}_\alpha(x,u)$ is strongly closed \cite[Thm. 3.7, p. 60]{brezis2010}.
%\footnote{That is, for any sequence in $\mathcal{R}_\alpha(x,u)$ that converges weakly to some $\xi \in L^2$, it holds that $\xi \in \mathcal{R}_\alpha(x,u)$.} 
%A convex subset of a Banach space is weakly closed if and only if it is strongly closed \cite[Thm. 3.7, p. 60]{brezis2010}, and $\mathcal{R}_\alpha(x,u)$ is a convex subset of $L^2$, a Banach space. %and hence, it suffices to show that $\mathcal{R}_\alpha(x,u)$ is strongly closed. 
%Let $(\xi_n)_{n \in \mathbb{N}} \subseteq \mathcal{R}_\alpha(x,u)$ converge strongly to $\xi^* \in L^2$. Since strong convergence implies weak convergence and by \cite[Thm. 2.5.1, Thm. 2.5.3, pp. 92-93]{ash1972}, it follows that $\xi^* \in \mathcal{R}_\alpha(x,u)$.
%i.e.,  $||\xi_n-\xi^*||_{L_2}\rightarrow 0$ as $n \rightarrow \infty$. Strong convergence implies weak convergence, and thus, $\lim_{n\rightarrow \infty} \int_S \xi_n(y) Q(\mathrm{d}y|x,u) = \int_S \xi^*(y) Q(\mathrm{d}y|x,u)$. Since $\int_S \xi_n(y) Q(\mathrm{d}y|x,u) = 1$ for all $n \in \mathbb{N}$, it follows that $\int_S \xi^*(y) Q(\mathrm{d}y|x,u) = 1$. Strong convergence implies the existence of a subsequence of $(\xi_n)_{n \in \mathbb{N}}$ that converges a.e. to $\xi^*$ \cite[Thm. 2.5.1, Thm. 2.5.3, pp. 92-93]{ash1972}. Thus, $\xi^*$ inherits the bounds of $(\xi_n)_{n \in \mathbb{N}}$ a.e., and $\xi^* \in \mathcal{R}_\alpha(x,u)$.

%every sequence in $\mathcal{R}_\alpha(x,u)$ has a subsequence that converges weakly to an element of $\mathcal{R}_\alpha(x,u)$.\footnote{$(\xi_i)_{i \in \mathbb{N}} \subseteq \mathcal{R}_\alpha(x,u)$ converges weakly to $\xi^* \in \mathcal{R}_\alpha(x,u)$ $\iff$ $\lim_{i \rightarrow \infty} \int_S \xi_i(y) f(y) Q(\mathrm{d}y|x,u) = \int_S \xi^*(y) f(y) Q(\mathrm{d}y|x,u)$ $\forall f \in L^2$.} 

%We show weak continuity first. A linear functional on a normed vector space is weakly continuous if and only if it is strongly continuous \cite[Prop. 2.5.3, p. 212]{Megginson}. Also, a linear functional on a normed vector space is strongly continuous if and only if it is bounded \cite[Prop. 5.2, p. 153]{folland2013real}. Since $\psi$ is a bounded linear functional on a normed space, it is weakly continuous.
